# Supplementary material for: Refined Commonsense Knowledge from Large-Scale Web Contents
Source: arXiv:2112.04596 source file (2022-06-23)
Supplement: Supplementary file 1 [file appendix.tex]

\appendices
\section{Crowdsourcing question templates}
\begin{table}[h]
    \centering
    \begin{tabular}{llll}
    \toprule
    \textbf{Dimension} & \textbf{Question} & \textbf{Options} \\
    \midrule
    Correctness & \textit{How often does this answer hold true?} & \begin{tabular}[c]{@{}l@{}}\textbf{3 - Always/Often} - the answer is always or often true\\ \textbf{2 - Sometimes/Likely} - it is sometimes or likely true\\ \textbf{1 - Farfetched/Never} - it is false or farfetched at best\\ \textbf{0 - Invalid} - it is invalid or makes no sense\end{tabular} \\
    \midrule
    % Saliency & \textit{\begin{tabular}[c]{@{}l@{}}Imagine you have 2 minutes time to explain\\ a kid about \textless{}subject\textgreater{}, would you mention\\ the following information?\end{tabular}} & \begin{tabular}[c]{@{}l@{}}\textbf{Absolutely} - the information is very interesting/important for that concept\\ \textbf{Probably} - it is quite good to know\\ \textbf{Maybe not} - it is not interesting or too obvious/uninteresting/boring\\ \textbf{Definitely not} - it is completely irrelevant/unimportant/wrong or makes no sense\end{tabular} \\
    Informativeness & \textit{How informative is the answer?} & \begin{tabular}[c]{@{}l@{}}\textbf{3 - Highly} - the answer provides very useful knowledge\\ \textbf{2 - Moderately} - the answer is moderately useful\\ \textbf{1 - Slightly} - the answer is slightly useful\\ \textbf{0 - Not at all} - the answer is too general or makes no sense\end{tabular} \\
    \bottomrule
    \end{tabular}
    \caption{Crowdsourcing question templates for commonsense QA evaluation.}
    \label{tab:mturk-qa}
\end{table}
